# Supplementary material for: Particle-Particle Random Phase Approximation for Predicting Correlated Excited States of Point Defects
Source: arXiv:2406.18515 ancillary file (2024-06-26)
Supplement: Supplementary file 1 [file supporting_information.pdf]

# Supporting Information:

## Particle-Particle Random Phase Approximation for Predicting Correlated Excited States of Point Defects

Jiachen Li,<sup>\*,†</sup> Yu Jin,<sup>‡</sup> Jincheng Yu,<sup>¶</sup> Weitao Yang,<sup>\*,¶</sup> and Tianyu Zhu<sup>\*,†</sup>

<sup>†</sup>*Department of Chemistry, Yale University, New Haven, Connecticut 06520, United States*

<sup>‡</sup>*Pritzker School of Molecular Engineering, University of Chicago, Chicago, Illinois 60637,  
United States*

<sup>¶</sup>*Department of Chemistry, Duke University, Durham, North Carolina 27708, United  
States*

E-mail: [jiachen.li@yale.edu](mailto:jiachen.li@yale.edu); [weitao.yang@duke.edu](mailto:weitao.yang@duke.edu); [tianyu.zhu@yale.edu](mailto:tianyu.zhu@yale.edu)

# 1 Details about geometry optimizations

We optimized the ground-state equilibrium geometries of point defect systems using density functional theory<sup>S1,S2</sup> (DFT) and the plane-wave pseudopotential method, as implemented in the Quantum ESPRESSO package,<sup>S3,S4</sup> by minimizing the nuclear forces below the threshold of 0.01 eV Å<sup>-1</sup>. Our study involved Kohn-Sham DFT calculations for the singlet ground states of point defect systems, specifically the <sup>1</sup>A<sub>1g</sub> ground state of VO in MgO and the <sup>1</sup>A<sub>1</sub> ground state of C<sub>B</sub>C<sub>N</sub> in 2D-hBN. For VC in diamond, two separate DFT calculations were performed to obtain the equilibrium geometry with the D<sub>2d</sub> and the T<sub>d</sub> symmetry. To obtain the geometry with the T<sub>d</sub> symmetry, each of the three degenerate *t*<sub>2</sub> KS orbitals was enforced to accommodate 2/3 of an electron. We used SG15 ONCV norm-conserving pseudopotentials<sup>S5,S6</sup> and the PBE<sup>S7</sup> functional with the plane-wave energy cutoff setting to 60 Ry.

# 2 Excitation energies of defects obtained from ppRPA

Table S1: Vertical excitation energies of VC in diamond obtained from ppRPA@PBE and ppRPA@B3LYP with supercell models containing 63 and 215 atoms. (*O*, *V*) means that *O* occupied orbitals and *V* virtual orbitals were used in the active space. The geometry of the <sup>1</sup>A<sub>1</sub> ground state and cc-pVDZ basis set were used. All values are in eV.

|                          | ppRPA@PBE                                      |                                               | ppRPA@B3LYP                                    |                                               |
|--------------------------|------------------------------------------------|-----------------------------------------------|------------------------------------------------|-----------------------------------------------|
|                          | <sup>1</sup> T <sub>2</sub> (D <sub>2d</sub> ) | <sup>1</sup> T <sub>2</sub> (T <sub>d</sub> ) | <sup>1</sup> T <sub>2</sub> (D <sub>2d</sub> ) | <sup>1</sup> T <sub>2</sub> (T <sub>d</sub> ) |
| supercell 63             | 1.43                                           | 1.38                                          | 1.70                                           | 1.62                                          |
| supercell 215 (200, 200) | 1.91                                           | 1.78                                          | 2.30                                           | 2.14                                          |
| supercell 215 (250, 250) | 1.84                                           | 1.71                                          | 2.22                                           | 2.05                                          |
| supercell 215 (300, 300) | 1.81                                           | 1.67                                          | 2.19                                           | 2.01                                          |
| supercell 215 (400, 400) | 1.78                                           | 1.64                                          | 2.15                                           | 1.96                                          |

Table S2: Vertical excitation energies of VO in MgO obtained from ppRPA@PBE and ppRPA@B3LYP with supercell models containing 63 and 215 atoms. ( $O$ ,  $V$ ) means that  $O$  occupied orbitals and  $V$  virtual orbitals were used in the active space. The geometry of the  $^1A_{1g}$  ground state and cc-pVDZ basis set were used. All values are in eV.

|                          | ppRPA@PBE  |            | ppRPA@B3LYP |            |
|--------------------------|------------|------------|-------------|------------|
|                          | $^1T_{1u}$ | $^3T_{1u}$ | $^1T_{1u}$  | $^3T_{1u}$ |
| supercell 63             | 5.05       | 3.91       | 5.23        | 3.97       |
| supercell 215 (200, 200) | 4.75       | 3.52       | 4.90        | 3.49       |
| supercell 215 (250, 250) | 4.76       | 3.53       | 4.92        | 3.51       |
| supercell 215 (300, 300) | 4.80       | 3.57       | 4.98        | 3.56       |
| supercell 215 (400, 400) | 4.82       | 3.60       | 5.01        | 3.60       |

Table S3: Vertical excitation energies of  $C_B C_N$  in h-BN obtained from ppRPA\*@PBE and ppRPA\*@B3LYP with the supercell model containing 128 atoms. ( $O$ ,  $V$ ) means that  $O$  occupied orbitals and  $V$  virtual orbitals were used in the active space. The geometry of the  $^1A_1$  ground state and cc-pVDZ basis set were used. All values are in eV.

|                          | ppRPA@PBE | ppRPA@B3LYP |
|--------------------------|-----------|-------------|
|                          | $^1A_1$   | $^1A_1$     |
| supercell 128 (200, 200) | 3.76      | 4.51        |
| supercell 128 (250, 250) | 3.76      | 4.52        |
| supercell 128 (300, 300) | 3.77      | 4.52        |
| supercell 128 (400, 400) | 3.77      | 4.52        |

### 3 Basis set convergence

Vertical excitation energies of VO in MgO obtained from ppRPA@PBE and ppRPA@B3LYP with cc-pVDZ and cc-pVTZ basis sets<sup>S8</sup> and the supercell model containing 63 atoms are tabulated in Table. S4. It shows that excitation energies obtained from ppRPA with cc-pVDZ and cc-pVTZ basis sets are very similar. The differences between the results of ppRPA using cc-pVDZ and cc-pVTZ are smaller than 0.02 eV. Thus, the cc-pVDZ basis set is used for ppRPA calculations in this work.

Table S4: Vertical excitation energies of VO in MgO obtained from ppRPA@PBE and ppRPA@B3LYP with cc-pVTZ basis set. ( $O$ ,  $V$ ) means that  $O$  occupied orbitals and  $V$  virtual orbitals were used in the active space. The geometry of the  $^1A_{1g}$  ground state and the supercell model containing 63 atoms were used. All values are in eV.

|            | ppRPA@PBE cc-pVDZ   |            | ppRPA@PBE cc-pVTZ   |            |
|------------|---------------------|------------|---------------------|------------|
|            | $^1T_{1u}$          | $^3T_{1u}$ | $^1T_{1u}$          | $^3T_{1u}$ |
| (200, 200) | 5.05                | 3.91       | 5.03                | 3.89       |
| (300, 300) | 5.05                | 3.91       | 5.03                | 3.89       |
|            | ppRPA@B3LYP cc-pVDZ |            | ppRPA@B3LYP cc-pVTZ |            |
|            | $^1T_{1u}$          | $^3T_{1u}$ | $^1T_{1u}$          | $^3T_{1u}$ |
| (200, 200) | 5.24                | 3.96       | 5.23                | 3.96       |
| (300, 300) | 5.23                | 3.96       | 5.22                | 3.97       |

### 4 Excitation energies of defect systems obtained from TDDFT

Table S5: Vertical excitation energies of VC in diamond obtained from TDDFT@PBE and TDDFT@B3LYP with supercell models containing 63 and 215 atoms. The geometry of the  $^1A_1$  ground state of  $D_{2d}$  symmetry was used. All values are in eV.

|                             | $^1T_2$ |
|-----------------------------|---------|
| TDDFT@PBE (supercell 63)    | 1.01    |
| TDDFT@PBE (supercell 215)   | 1.19    |
| TDDFT@B3LYP (supercell 63)  | 1.07    |
| TDDFT@B3LYP (supercell 215) | 1.30    |

Table S6: Vertical excitation energies of VO in MgO obtained from TDDFT@PBE and TDDFT@B3LYP with supercell models containing 63 and 215 atoms. The geometry of the  $^1A_{1g}$  ground state was used. All values are in eV.

|                             | $^1T_{1u}$ | $^3T_{1u}$ |
|-----------------------------|------------|------------|
| TDDFT@PBE (supercell 63)    | 5.02       | 3.79       |
| TDDFT@PBE (supercell 215)   | 3.86       | 3.29       |
| TDDFT@B3LYP (supercell 63)  | 5.35       | 3.92       |
| TDDFT@B3LYP (supercell 215) | 4.60       | 3.57       |

Table S7: Vertical excitation energies of  $C_B C_N$  in h-BN obtained from TDDFT@PBE and TDDFT@B3LYP with the supercell model containing 128 atoms. The geometry of the  $^1A_1$  ground state was used. All values are in eV.

|                             | $^1A_1$ |
|-----------------------------|---------|
| TDDFT@PBE (supercell 128)   | 4.03    |
| TDDFT@B3LYP (supercell 128) | 4.63    |

## References

- (S1) Hohenberg, P.; Kohn, W. Inhomogeneous Electron Gas. *Phys. Rev.* **1964**, *136*, B864–B871.
- (S2) Parr, R. G.; Weitao, Y. *Density-Functional Theory of Atoms and Molecules*; Oxford University Press, 1989.
- (S3) Giannozzi, P.; Barone, O.; Bonfà, P.; Brunato, D.; Car, R.; Carnimeo, I.; Cavazzoni, C.; de Gironcoli, S.; Delugas, P.; Ferrari Ruffino, F.; Ferretti, A.; Marzari, N.; Timrov, I.; Urru, A.; Baroni, S. Quantum ESPRESSO toward the Exascale. *J. Chem. Phys.* **2020**, *152*, 154105.
- (S4) Carnimeo, I.; Affinito, F.; Baroni, S.; Barone, O.; Bellentani, L.; Bertossa, R.; Delugas, P. D.; Ruffino, F. F.; Orlandini, S.; Spiga, F.; Giannozzi, P. Quantum ESPRESSO: One Further Step toward the Exascale. *J. Chem. Theory Comput.* **2023**, *19*, 6992–7006.
- (S5) Hamann, D. R. Optimized Norm-Conserving Vanderbilt Pseudopotentials. *Phys. Rev. B* **2013**, *88*, 085117.
- (S6) Schlipf, M.; Gygi, F. Optimization Algorithm for the Generation of ONCV Pseudopotentials. *Computer Physics Communications* **2015**, *196*, 36–44.
- (S7) Perdew, J. P.; Burke, K.; Ernzerhof, M. Generalized Gradient Approximation Made Simple. *Phys. Rev. Lett.* **1996**, *77*, 3865–3868.
- (S8) Dunning, T. H. Gaussian Basis Sets for Use in Correlated Molecular Calculations. I. The Atoms Boron through Neon and Hydrogen. *J. Chem. Phys.* **1989**, *90*, 1007–1023.
